# Supplementary material for: System-Level Safety Monitoring and Recovery for Perception Failures in Autonomous Vehicles
Source: arXiv:2409.17630 source file (2024-10-06)
Supplement: Supplementary file 1 [file appendix.tex]

Possibly mention the details of the FRT computation, a few more examples, and the confusion matrix.
